# Supplementary material for: Ghosts of Order on the Frontier of Chaos
Source: arXiv:1610.09170 source file (2016-10-28)
Supplement: Supplementary file 1 [file apmPrinth.tex]

\begin{verbatim} 


\end{verbatim}
