# Supplementary material for: Ghosts of Order on the Frontier of Chaos
Source: arXiv:1610.09170 source file (2016-10-28)
Supplement: Supplementary file 2 [file apmSpecialh.tex]

\begin{verbatim} 
# define MAX_TRIG_TERMS  100
# define DFLT_TRIG_DP    20

# define PI_DP	    (sizeof(pi_str) / sizeof(char) - 3)

# ifndef YES
# define YES  1
# define NO   0
# endif 

# ifndef m_swap
# define m_swap(x,y,t)	(t=x, x=y, y=t) 
# endif 

extern APM    zero, one, two ;
extern APM    pi, two_pi, half_pi, threeHalf_pi, eighths_2pi[8] ;
extern APM    Theta, scratch, xMod2pi, Theta_sq, Answer ;
extern APM    Factrl, coef, apmOrder ;
extern APM    approx[2], diff, ub_diff ;
extern int    trig_dp, specialsInit ;
extern int    trig_terms, dp_lost ;
extern char   pi_str[] ;
\end{verbatim}
